# Supplementary material for: Option-Critic in Cooperative Multi-agent Systems
Source: arXiv:1911.12825 source file (2020-03-19)
Supplement: Supplementary file 1 [file supplementary.tex]

\setcounter{section}{0}
\pagenumbering{roman}
\setcounter{page}{1}
\section*{\Large{Supplementary material for \emph{Option-critic in cooperative multi-agent systems}}}
\section{Definitions}\label{supp:definitions}
\begin{definition}[Dec-POMDP]\label{def:dec-POMDP}
\begin{itemize}
  \item $\ALPHABET S$ is a finite set of states of the world (environment + agents).
  \item $\ALPHABET A = \ALPHABET A^1 \times \dots \times \ALPHABET A^J$ is a finite set of joint actions, where $\ALPHABET A^j$, $j \in \ALPHABET J$ is the set of actions taken by Agent~$j$. At time $t$, \emph{joint action} $\mathbf a_t \in \ALPHABET A$ implies $\mathbf a_t = (a^1_t, \dots, a^J_t)$ where $a^j_t \in \ALPHABET A^j$, $j \in \ALPHABET J$.
  \item $\PR: \ALPHABET S \times \ALPHABET A \times \ALPHABET S \rightarrow [0,1]$ is a transition function. For any $t'>t$, $\PR(\mathbf{s}_{t'} = \mathbf{s'}\,|\, \mathbf s_t = \mathbf s, \mathbf a_t = \mathbf a)$ is the probability of the outcome state $\mathbf{s}_{t'} = \mathbf{s'}$ when the joint-action $\mathbf{a}_t = \mathbf{a}$ is taken in joint-state $\mathbf{s}_t = \mathbf{s}$.
  \item $R$ is a reward function. For any $t'>t$, $R(\mathbf{s}, \mathbf a, \mathbf{s'})$ is the reward obtained from taking joint-action $\mathbf a_t = \mathbf a$ is joint-state $\mathbf s_t = \mathbf s$ and transitioning to joint-state $\mathbf s_{t'} = \mathbf{s'}$.
  \item $\ALPHABET O = \ALPHABET O^1 \times \dots \times \ALPHABET O^J$ is the finite set of all observations, where $\ALPHABET O^j$ is the finite set of observations of Agent~$j$, $j \in \ALPHABET J$.
  \item $\eta: \ALPHABET S \times \ALPHABET A \rightarrow [0,1]$ is the observation function $\eta(\mathbf o | \mathbf s, \mathbf a)$ is the joint-probability that all agents observe the  $\mathbf o_t = \mathbf o$ when the agents
execute the joint-action $\mathbf a_{t-1} = \mathbf a$ to arrive at the  joint-state $\mathbf s$. Here $\mathbf o = (o^1,\dots, o^J)$, $\mathbf o \in \ALPHABET O$, denotes the realization of the joint-observation $\mathbf o_t$ of all agents at time $t$.
\item $I \in \Delta(\ALPHABET S)$ is the initial state distribution at stage $t = 0$, where the simplex $\Delta(\ALPHABET S)$ denotes the space of probability distributions on $\ALPHABET S$. 
  \end{itemize}
\end{definition}

Some special cases of the generic $J$-agent Dec-POMDP~\cite{Oliehoek:book,Becker:2004} are defined as follows.
\begin{definition}[Special Dec-POMDPs]\label{def:specialDec-POMDP}
\begin{itemize}
  \item \textbf{with Factored state space}: if the state space $\ALPHABET S$ of the world can be factored into components $\ALPHABET S^0$ and $\ALPHABET S^j$, $j \in \ALPHABET J$, with $\ALPHABET S = \ALPHABET S^0 \times \ALPHABET S^1 \times \dots \times \ALPHABET S^J$. Here $\ALPHABET S^0$ consists of the part of world states that is not affected by the agents and $\ALPHABET S^j$, $j \in \ALPHABET J$, are parts of the world states that are affected by Agent~$j$. We denote by $(\hat s^j_t, a^j_t, y^j_t)$ as the local state, action and observation of Agent $j$, with their corresponding realizations $(\hat s^j, a^j, o^j)$. Here $\hat s^j \in \ALPHABET S^0 \times \ALPHABET S^j$. Note that when $\ALPHABET S^0 = \varnothing$, $\hat s^j_t = s^j_t$ for all $j \in \ALPHABET J$.
%   \item \textbf{Factored and transition independent}: if there exist local transition probability maps $P^j$, $j \in \ALPHABET J$, such that for any $t' > t$:
%   \[
%   \PR(s^0_{t'} = s^{'0}\,|\, s^0_t = s^0, \mathbf{s}_t = \mathbf{s}, \mathbf{a}_t = \mathbf{a}) 
%   = P^0(s^0_{t'} =  s^{'0}\,|\,s^0_t = s^0),
%   \]
%   and for any $j \in \ALPHABET J$,
%   \[
%      \PR(s^j_{t'} = s^{'j}\,|\, s^0_t = s^0, \mathbf{s}_t = \mathbf{s}, \mathbf{a}_t = \mathbf{a}) 
%       =
%                             %   & = \begin{cases}     P^0(s^0_t = s^{'0}\,|\, ss^0), & \mbox{if $j = 0$}\\
%                                   P^j(s^j_{t'} = s^{'j}\,|\, \hat s^j_t = \hat s^j, a^j_t = a^j).
%                                   %\end{cases}
%   \]
%   This implies for any realization $\mathbf{s'} = (s^{'1},\dots,s^{'J})$ of the joint-state $\mathbf s_{t'}$ at time $t' > t$,
%   \[
%     \PR(s^0_{t'} = s^{'0}, \mathbf{s}_{t'} = \mathbf s'\,|\, s^0_t = s^0, \mathbf{s}_t = \mathbf s, \mathbf{a}_t = \mathbf{a}) 
%      = \prod_{j = 0}^J P^j(s^j_{t'}=s^{'j}\,|\,  \hat s^j_{t}=s^{j}),
%   \]
% where we used the fact $\hat s^0_t = s^0_t$.
\item \textbf{with Factored action space}: if the \emph{joint-policy} $\pi$ is made up of component sub-policies $\pi^j$, such that $\pi^j: \ALPHABET O^j \rightarrow \PR(a^j_t)$, $j \in \ALPHABET J$.
  \item \textbf{Locally fully observable}: if for all $o^j$, there exists $s^j$ such that $\PR(s^j\,|\,o^j) = 1$.
  \item \textbf{Factored and reward independent}: if there exist local reward functions $R^j$, $j \in \ALPHABET J$ such that 
  \[
  R\left(\mathbf s, \mathbf a, \mathbf{s'} \right) 
  = \sum_{j \in \ALPHABET J} R^j(s^j,a^j,s^{'j}).
  \]
  \end{itemize}
\end{definition}
% The local full observability makes the system we consider in this paper a $J$-agent Markov decision process (Dec-MDP), which is a special case of Dec-POMDP as defined below.
% \begin{definition}[Dec-MDP]\label{def:dec-mdp}
% A $J$-agent Dec-MDP is a special case of a $J$-agent Dec-POMDP with the following property:
% \begin{itemize}
%     \item  Joint full observability: the tuple of observations made
%     by the agents together fully determine the current state. If $\eta(\mathbf s, \mathbf a, \mathbf{s'}, \mathbf y) > 0$ then for any $t'>t$, $P(\mathbf s_{t'} = \mathbf{s'}\,|\,\mathbf y_t = \mathbf y) = 1$.
% \end{itemize}
% \end{definition}
\section{Proof of Lemma~\ref{lemma:tilde-h}}\label{supp:proof_Lemma-tilde-h}
At any instant $t$, the common-observation $\boldsymbol{\tilde o}_t$ depends on the broadcasting, which in turn depends on the current observation $o^j_t$\footnote{In case of locally fully observable agents the broadcasting depends on the current state $s^j_t$ or embedding $e^j_t$ of each agent.} and the current option $\omega^j_t$. Note that $\mathbf o_t \sim \eta(\mathbf o_t | \mathbf s_t, \mathbf a_{t-1})$ and $\mathbf a_{t-1}$ is absorbed in $b^c_t$ via conditioning by $\boldsymbol{\omega}_{t-1}$ and because $I^c_{t-1} \subset I^c_t$. Thus, we have by~\eqref{eq:mu_t_psi_tilde} that $\mathbf o_t$ is absorbed by $\mu_t$. Moreover, since the joint-options $\boldsymbol{\omega}_t$ are generated by the joint option-policies $\mu_t$, the function $\tilde h_t$ exists. A particular expression for $\tilde h_t$ is given by~\eqref{eq:tilde-h}.

We show the equality of~\eqref{eq:prob_o_coordinated_sys} by shedding off \emph{irrelevant information}. First, note that the information captured in $\mathbf o^\dagger_{1:t}$ and $\boldsymbol{\tilde o}_{1:t-1} \eqqcolon \mathbf o^\dagger_t$ are the same. So, $\mathbf o^\dagger_{1:t-1}$ can be considered as redundant (and thus irrelevant) information and can hence be removed from conditioning. The common-observation $\boldsymbol{\tilde o}_t$ depends on the joint-state $\mathbf s_t$ and the joint option-policy $\mu_t$ (through $\tilde h_t$). So, when conditioned by $\mu_t$, $\mu_{1:t-1}$ does not give any additional information about $\boldsymbol{\tilde o}_t$ and can thus be removed from conditioning. In particular, we have
\begin{align*}
    &\PR(\mathbf o^\dagger_{t+1} = \mathbf o^\dagger\,|\,  \mathbf o^\dagger_{1:t}, \mu_{1:t}) \\
    & = \PR(\boldsymbol{\tilde o}_{1:t}= \mathbf o^\dagger\,|\,  \boldsymbol{\tilde o}_{1:t-1}, \mu_{1:t})
    = \PR(\boldsymbol{\tilde o}_{1:t}= \mathbf o^\dagger\,|\,  \boldsymbol{\tilde o}_{1:t-1}, \mu_t)\\
     & = \PR(\mathbf o^\dagger_{t+1} = \mathbf o^\dagger \,|\,  \mathbf o^\dagger_t, \mu_t).
\end{align*}
This completes the proof.

\section{Proof of Lemma~\ref{lemma:info-state-option}}\label{supp:proof_lemma_info-state}
The proof follows an argument similar to~\cite{KumarVaraiya:1986} for primitive actions. In particular,
\begin{enumerate}
  \item The equality of Part~1) readily holds from the fact that $b^c_t$ is measurable by $\{\boldsymbol{\tilde o}_{1:t-1}, \boldsymbol{\omega}_{1:t-1}\}$ and so conditioning by $\{\boldsymbol{\tilde o}_{1:t-1}, \boldsymbol{\omega}_{1:t-1}\}$ is the same as conditioning by $b^c_t$.
  \item From~\eqref{eq:belief-Bayes-update-options} we can write 
  \[
  \PR(b^c_{t+1}\,|\, \boldsymbol{\tilde o}_{1:t-1}, \boldsymbol{\omega}_{1:t-1}) = \PR(\mathbf s_{t+1}\,|\, \boldsymbol{\bar o}_{1:t-1}, \boldsymbol{\omega}_{1:t-1})\IND(\boldsymbol{\bar o}_{1:t-1} = \boldsymbol{\tilde o}_{1:t-1}).
  \]
  Then the equality follows from the fact that $b^c_t$ is measurable by $\{\boldsymbol{\tilde o}_{1:t-1}, \boldsymbol{\omega}_{1:t-1}\}$ and that conditioning on $b^c_t$ is same as conditioning on $\{\boldsymbol{\tilde o}_{1:t-1}, \boldsymbol{\omega}_{1:t-1}\}$ (as is shown by part~1).
  \item We have by the definition of option
  \begin{align*}
  &\EXP [r^{\boldsymbol{\omega}_t}(\mathbf s_t)\,|\, \boldsymbol{\tilde o}_{1:t-1}, \boldsymbol{\omega}_{1:t}]\\
  & = \sum_{\boldsymbol{\mathrm{br}}_t\in \{0,1\}^J}
  \sum_{\mathbf a_t \in \ALPHABET A}
  \pi^{b,\boldsymbol{\omega}_t}_t(\boldsymbol{\mathrm{br}}_t|\mathbf o_t)\pi^{\boldsymbol{\omega}_t}_t(\mathbf a_t|\mathbf o_t) \\
  &\hskip 4em \times f_t(\mathbf o_t, \mathbf s_t, \boldsymbol{\omega}_{t-1}) \EXP[r^{\mathbf a_t, \boldsymbol{\mathrm{br}}_t}(\mathbf s_t)\,|\,\boldsymbol{\tilde o}_{1:t-1}, \boldsymbol{\omega}_{1:t-1}]\\
  &= \sum_{\boldsymbol{\mathrm{br}}_t\in \{0,1\}^J} \sum_{\mathbf a_t \in \ALPHABET A}
  \pi^{b,\boldsymbol{\omega}_t}(\boldsymbol{\mathrm{br}}_t|\mathbf o_t)\pi^{\boldsymbol{\omega}_t}_t(\mathbf a_t|\mathbf o_t) f_t(\mathbf o_t, \mathbf s_t, \boldsymbol{\omega}_{t-1})\\
  & \hskip 8em \times \sum_{\mathbf s_t \in \ALPHABET S} r^{\mathbf a_t,\boldsymbol{\mathrm{br}}_t }(\mathbf s_t) \PR(\mathbf s_t \,|\,\boldsymbol{\tilde o}_{1:t-1}, \boldsymbol{\omega}_{1:t-1})\\
  & \stackrel{(a)}{=} \EXP [r^{\boldsymbol{\omega}_t}(\mathbf s_t)\,|\, b^c_t, \boldsymbol{\omega}_t],
  \end{align*}
  where $(a)$ holds by the definition of $b^c_t$.
  \end{enumerate}
  where $f_t$ is given by~\eqref{eq:f_t-recursive}.
%   \begin{align*}
%   f_t(\mathbf o_t, \mathbf s_t, \boldsymbol{\omega}_{t-1}) &\DEFINED \sum_{a_{t-1} \in \ALPHABET A} \eta(\mathbf o_t|, \mathbf a_{t-1},\mathbf s_t)\pi^{\boldsymbol{\omega}_{t-1}}_t(\mathbf a_{t-1}|\mathbf o_{t-1})\\
%   & \hskip 6em \times f_{t-1}(\mathbf o_{t-1}, \mathbf s_{t-1}, \boldsymbol{\omega}_{t-2}).
%   \end{align*}
  This completes the proof of the lemma. 

\section{Proof of Lemma~\ref{lemma:Q-star-contraction}}\label{supp:proof-contraction}
We prove the contraction of $\ALPHABET B^*$. That $\ALPHABET B^{\mu_t}$ is a contraction can be shown similarly. 

We begin by noting that the supremum in the definition of the sup-norm can be replaced by maximum since $\ALPHABET S$ is finite. Then, we have 
\begin{align*}
&\|\ALPHABET B^* Q^*\|_\infty \\
&= \gamma \max_{b^c_t \in \Delta(\ALPHABET S)}\max_{\boldsymbol{\omega}_t \in \Omega} \sum_{\mathbf s_t \in \ALPHABET S}\Big[ \sum_{\boldsymbol{\mathrm{br}}_t \in \{0,1\}^J}\sum_{\mathbf a_t \in \ALPHABET A}
\pi^{b,\boldsymbol{\omega}_t}_t(\boldsymbol{\mathrm{br}}_t|\mathbf o_t)\\ 
&\hskip 8em \times \pi^{\boldsymbol{\omega}_t}_t(\mathbf a_t | \mathbf o_t) f_t(\mathbf o_t, \mathbf s_t, \boldsymbol{\omega}_{t-1})\\
& \hskip 2em \times 
 \Big( \sum_{\mathbf s_{t+1} \in \ALPHABET S} b^c_{t+1}(\mathbf s_{t+1}) p^{\mathbf a_t}(\mathbf s_t,\mathbf s_{t+1}) U^*(\mathbf s_{t+1}, \boldsymbol{\omega}_t)\Big)\Big]b^c_t(\mathbf s_t)\\
& \stackrel{(a)}{\le} \gamma \max_{b^c_t \in \Delta(\ALPHABET S)}\|Q^*\|_\infty \sum_{\mathbf s_t \in \ALPHABET S} \Big[\sum_{\boldsymbol{\mathrm{br}}_t \in \{0,1\}^J} \sum_{\mathbf a_t \in \ALPHABET A}
\pi^{b,\boldsymbol{\omega}_t}_t(\boldsymbol{\mathrm{br}}_t|\mathbf o_t)\\
 & \hskip 2em \times \pi^{\boldsymbol{\omega}_t}_t(\mathbf a_t | \mathbf s_t) \Big( \sum_{\mathbf s_{t+1} \in \ALPHABET S} b^c_{t+1}(\mathbf s_{t+1}) p^{\mathbf a_t}(\mathbf s_t,\mathbf s_{t+1})\Big)\Big]b^c_t(\mathbf s_t)\\
& \stackrel{(b)}{\le} \gamma \|Q^*\|_\infty,
\end{align*}
where $(a)$ follows from~\eqref{eq:U-mu-b}--\eqref{eq:U-star-b-Q-star-b} by using Cauchy-Schwartz inequality and the definition of sup-norm and from the fact that $f_t(\mathbf o_t, \mathbf s_t, \boldsymbol{\omega}_{t-1}) \le 1$. $(b)$ holds due to the fact that 
\begin{align*}
&\sum_{\mathbf s_t \in \ALPHABET S} \Big[\sum_{\boldsymbol{\mathrm{br}}_t \in \{0,1\}^J} \sum_{\mathbf a_t \in \ALPHABET A} \pi^{b,\boldsymbol{\omega}_t}_t(\boldsymbol{\mathrm{br}}_t|\mathbf o_t)\pi^{\boldsymbol{\omega}_t}_t(\mathbf a_t| \mathbf s_t)\\
& \hskip 4em \times \Big( \sum_{\mathbf s_{t+1} \in \ALPHABET S} b^c_{t+1}(\mathbf s_{t+1}) p^{\mathbf a}(\mathbf s_t, \mathbf s_{t+1})\Big)\Big]b^c_t(\mathbf s_t) \\
& \le 1.
\end{align*}
The last inequality implies contraction since $\gamma \in (0,1)$. This completes the proof of the lemma.

\section{Proof of Theorem~\ref{thm:prescription-based-optimality}}\label{supp:proof-thm-DP}
\begin{enumerate}
\item The common information approach~\cite{NMT:partial-history-sharing} converts a Dec-MDP into an  equivalent centralized POMDP, where there is a single decision maker, a \emph{coordinator}, who observes the common information $\{\boldsymbol{\tilde o}_{1:t-1}, \boldsymbol{\omega}_{1:t-1}\}$ and prescribes joint-option policy $\mu_t$. Since the system is a POMDP with $b^c_t$ acting as a state, the state-value $V^{\mu_t}(b^c_t)$ for a given joint option-policy $\mu_t$ satisfies the Bellman equation given by~\eqref{eq:V-mu}.
%   \begin{equation}
%   V^{\mu_t}(b^c_t) = \sum_{\mathbf o \in \ALPHABET O} \mu_t(\mathbf o|b^c_t)\Bigg[r^{\mathbf o}(b^c_t)] 
%   + \gamma \EXP \Big[\sum_{\mathbf y \in \Omega} \PR(\mathbf y|b^c_t, \mathbf o)V^{\mu_t}(b^c_{t+1}) \,\Bigm|\, b^c_t\Big]\Bigg] \label{eq:V-mu}.
%   \end{equation}
  
It can be shown following standard results for
POMDP that~\eqref{eq:V-mu} is a contraction and hence there exists a unique bounded solution $V^{\mu_t}$.  

Since the set of probability measures on finite spaces is finite, we can use $\max$ instead of $\sup$ in defining the optimal state-value $V^*$ in~\eqref{eq:V-option}. Thus, we have  
\[
V^*(b^c_t) \DEFINED \max_{\mu_t \in \ALPHABET M^+} V^{\mu_t}(b^c_t).
\]
Since maximum of a bounded function over a finite set is bounded, we have that $V^*$ is unique and bounded.
\item Let $\mu^* \in \ALPHABET M$ be a time-homogeneous Markov joint option-policy. We need to show that such a $\mu^*$ exists, which is optimal. If it does, then  $V^* =  V^{\mu^*}$. The existence of a time-homogeneous Markov joint-option policy, which achieves the optimal state-value $V^*$, follows from \emph{Blackwell optimality}.\footnote{A well-known result by Blackwell~\cite{blackwell1962} states that, in any MDP with finitely many states and finitely many actions with discounted reward, there is a pure stationary (time-homogeneous) strategy that is optimal, for every discount factor
close enough to one. This property is referred to as
\emph{Blackwell optimality}. Extension of Blackwell optimality holds for discounted infinite horizon POMDPs. See~\cite[Theorem~2.6.1]{krishnaArxiv2015} for details.}

Now,  following Proposition~\ref{prop:prescription} we can restrict our attention to the set of joint option-policies $M^{\psi, b^c_t}$ where any $\tilde \mu \in M^{\psi, b^c_t}$ is a function of the  coordination rule  $\psi$ and the common information based belief $b^c_t$. Thus, we have that 
\[
V^*(b^c_t) = \max_{\mu \in \ALPHABET M \cap \tilde M^{\psi, b^c_t}} V^\mu(b^c_t).
\]
This completes the proof. 
\end{enumerate}

\input{AAMAS20/OE_OI.tex}

\section{Details for the proof of Theorem~\ref{thm:algo-convergence}}\label{supp:thm_proof_convergernce}
It is well established that for a single-agent setup, temporal difference with policy gradient converges to the optimal option-value $Q^*$~\cite{Bacon2017TheOA}. In order to prove Theorem~\ref{thm:algo-convergence}, we have to show in addition that such a convergence to $Q^*$ is achieved in the multi-agent setup with the \emph{distributed} option-critic. For that matter, we first need some definitions given as follows. 
\subsubsection{Some definitions}
\begin{definitionS}[Nash equilibrium]
\label{defS:nash}
In a static (one-shot) team problem, also known as \emph{Identical Payoff Game}~\cite{PeshkinEtAl}, a \emph{Nash equilibrium} point is a joint policy $\pi^* = \mathrm{vec}(\pi^{1*}, \dots, \pi^{J*})$, such that for a belief $b$
\[
  V^{\pi^*}(b) \ge V^{\tilde \pi^*}(b),
\]
where $\tilde \pi^*$ denotes the joint-policy with \emph{unilateral deviation}. In particular, it denotes the joint-policy where one agent~$j$ follows policy $\pi^j$, different from $\pi^{j*}$, and all other agents$-j$ follow policies $\pi^{-j*}$. An implication of Nash equilibrium is that there is no incentive for any agent to unilaterally deviate from the equilibrium. 
\end{definitionS}
When the inequality in Definition~\ref{defS:nash} is strict, the equilibrium is called a \emph{strict Nash}. If a static game has more than one Nash equilibrium, we call the Nash equilibrium with highest value the \emph{optimal} Nash.

\begin{definitionS}[Subgame]
\label{defS:subgame}
A dynamic game (alternatively, an \emph{extensive-form game}) has a part that could be considered as a smaller game in itself; such a smaller game that is embedded in a larger game is called a \emph{subgame}. 
\end{definitionS}
In a dynamic game (played over time), the game at each instant (aka \emph{stage}) can be thought of a subgame.

A \emph{subgame perfect Nash equilibrium} is a refinement of a Nash equilibrium used in dynamic games. The definition of such an equilibrium is given below.
\begin{definitionS}[Subgame perfect Nash equilibrium]
\label{defS:SPNE}
A Nash equilibrium is said to be subgame perfect if an only if it is a Nash equilibrium in every subgame of a game.
\end{definitionS}
 Thus, in the context of a dynamic game, a joint-policy profile $\mu^*$ is called a \emph{subgame perfect Nash equilibrium} (or simply \emph{subgame perfect equilibrium}) if it represents a Nash equilibrium of every subgame of the original game. 

 If a dynamic game has more than one subgame perfect equilibrium, we call the subgame perfect equilibrium with highest value the \emph{optimal} subgame perfect Nash.

% \subsubsection{Proof of Theorem~\ref{thm:algo-convergence}}\label{subsec:proof_thm2}
% It has been established that every discounted stochastic game (which includes a static version of our problem) has at least one Nash equilibrium~\cite{HuWellman1998}. We first prove the following lemma.
% \begin{lemmaS}\label{lemmaS:DOC-SPNE}
% Cooperative Dec-POMDP planning with options leads to local optima. 
% \end{lemmaS}

%\begin{proof}
\section{Proof of Lemma~\ref{lemma:DOC-SPNE}}\label{supp:lemma-local-optima}
Let the tuple $(\pi^{j*}, \pi^{b,j*}, \beta^{j*})$ denote the action-policy, broadcast policy and the termination probability of Agent~$j$ parameterized by $(\theta^j, \epsilon^j, \varphi^j)$, as obtained by Algorithm~\ref{alg:DOI}. Let $\omega^*$ denote the joint option, $\boldsymbol{\omega}^* \DEFINED (\omega^{1*}, \dots, \omega^{J*})$, where option $\omega^{j*}$ of Agent~$j$, $j \in \ALPHABET J$, incorporates $(\pi^{j*}, \pi^{b,j*}, \beta^{j*})$. Also, denote by $\boldsymbol{\tilde \omega}^*$ an option with a \emph{unilateral deviation} from $\boldsymbol{\omega}^*$ (the concept of unilateral deviation is introduced in Definition~\ref{defS:nash}). 

The \emph{joint gradient descent} method of the planning problem that solves the dynamic program approximately (using methods such as \emph{Value Iteration} or \emph{Policy Iteration}) leads to the local optima. One can show using backward induction on the dynamic program (as is given by Theorem~\ref{thm:prescription-based-optimality}) that at each iteration $k$, for any common belief $b^c_k$ and option-policy $\mu$, such an optimum, denote it by $\boldsymbol{\omega}^*$, is such that 
\[
  Q^\mu(b^c_k, \boldsymbol{\omega}^*) > Q^\mu(b^c_k, \boldsymbol{\tilde \omega}^*),
\] 
and thus $\boldsymbol{\omega}^*$ is an optimal Nash. Following~\cite[Theorem~2]{PeshkinEtAl}, at every stage of the dynamic cooperative game, the \emph{distributed gradient descent} leads to optimal Nash (if there are more than one Nash equilibria, the one with highest option-value is chosen). Thus, for the dynamic cooperative game, the distributed gradient descent leads to subgame perfect Nash. Moreover, for factored agents,  distributed gradient descent is equivalent to joint gradient descent~\cite[Theorem~1]{PeshkinEtAl}, thus leading to local optima. This completes the proof of the lemma. %\qedhere 
